# Supplementary material for: Scalable Topical Phrase Mining from Text Corpora
Source: arXiv:1406.6312 source file (2014-11-19)
Supplement: Supplementary file 1 [file appendix.tex]

%!TEX root = ToPMine.tex
\section{Appendix}
\label{sec:appendix}
